# Supplementary material for: Quantum transport simulations in a programmable nanophotonic processor
Source: arXiv:1507.03406 source file (2020-01-28)
Supplement: Supplementary file 1 [file supp_info.pdf]

# Supplemental Material for Bosonic transport simulations in a large-scale programmable nanophotonic processor

July 1, 2015

## 1 PNP Calibration

Slight edge-wall roughness results in scattering that gives rise to small phase differences between two arms of a given reconfigurable beamsplitter (RBS) or (Mach-Zehnder interferometer). For a single RBS, this phase differential could be calibrated by simply measuring the power splitting ratio. However, there are many paths along which light can split and recombine in the PNP — significantly complicating the calibration process.

We calibrate the internal phase differential of each MZI by using a hill-climbing optimization algorithm that acts on the internal phase shifters, routing ‘wires’ of light through each MZI in the array. Once a wire was routed, the algorithm would monitor the power on the detector the wire routed towards. By modulating the internal phase shifters of each MZI composing the wire, all individual internal phase differentials could be obtained as a function of phase shifter bias voltage. An example of the measurements required to calibrate the internal phase differentials and phase versus bias voltage curves for each MZI along the edge of a single-input light cone is shown in Fig. 1.

To determine the phase differences between paths composed of multiple interferometers, we looked at the smallest interferometers we could construct using multiple individual interferometers — a meta-interferometer (See Fig. 1). We then used a similar method as for the single-MZIs (monitor a photodiode and then sweep the internal phases of the interferometer) to obtain the phase differentials for the meta-MZIs. Based on the meta-interferometer phase differentials, we were able to compute the settings necessary to produce a known unitary transformation both in simulation and in practice.

## 2 Experimental Setup

Our system has 213 thermo-optic phase shifters that require voltages from 0 to 10 volts and approximately 10 mA of current each. Electrical systems meeting these requirements at such a large scale do not exist in monolithic commercial form.

Such large systems do not exist in a monolithic commercial form, so we developed our own solution, which we call a Bias printed circuit board (PCB) as indicated in Fig. 2. Each channel is capable of sourcing tens of mA of current from 0 to 12 volts with 16-bit resolution (183  $\mu$ V discretization).

We also developed a custom 12-channel array of photodiodes with amplification circuitry and analog-to-digital conversion on a monolithic PCB. Each channel has approximately 40 dB dynamic range. The Detector Array PCB is shown schematically in Fig. 2.

In order to coordinate phase-write and output-read commands for the PNP, we employed a 72 MHz microcontroller which acted as a bridge between the Bias PCB, Detector Array PCB and a computer, as shown in Fig. 2. The computer sends a vector to the microcontroller containing the phase settings we would like to program into the PNP. The microcontroller then sends a command to the Bias PCB which then asserts requested voltage settings. Subsequently, the microcontroller issues a read command to the Photodiode Array PCB. The Photodiode Array PCB reads all channels and then returns a vector containing the measurements.

The PNP has a large density of electronic probe pads; there are 240, each measuring 80 by 80  $\mu$ m<sup>2</sup> at 100  $\mu$ m pitch. In order to contact each of these probe pads, we leveraged probe card technology from the volume semiconductor test industry. We employed two probe cards, each with 120 electrical contact pins, which contacted the system from either side.

### 3 Asymmetric Transport Correction

Modulating  $\phi_1$ , the upper output phase shifter in the RBS, throughout the PNP results in the asymmetric quantum walk transport distributions. In Fig. 3, we plot a computer simulation of  $\langle |\Psi(x, t_f)|^2 \rangle$  with all conditions identical to those in the main text, except that we only modulate  $\phi_1$ . These data show an asymmetric response to static and dynamic noise, specifically between modes 5 and 10—an artifact of modulating only the top phase shifter. To correct for this, we modulate  $\phi_1$  in the upper half of the array and  $\phi_2$  in the lower half of the array. This issue has not been explored in literature, to our knowledge, since it has not been readily possible to examine all static and dynamic disorder conditions under a large number of realizations.

### 4 Transport optimum

As noted in the main text, we predict that transport optima should exist for statically disordered quantum walks as dynamic disorder is introduced. We simulated at 15 time-step version of the PNP using the same settings as the main text; state preparation is identical,  $\phi_1$  is modulated in the top half of the array, and  $\phi_2$  is modulated in the bottom half of the array.

Fig. 4 shows the quantum transport space for the 30 modes of a simulated 15 time-step PNP. We simulated 100 realizations for each level of static and dynamic disorder with  $c_{td}, c_{tid} \in 0, 1$  in 20 evenly spaced samples (totaling 400 levels of disorder). Waveguide modes are indicated in the bottom right corner of each subplot. Modes 8, 9, 10, 21, 22, 23 each show transport optima for a given level of static disorder as dynamic disorder is introduced.

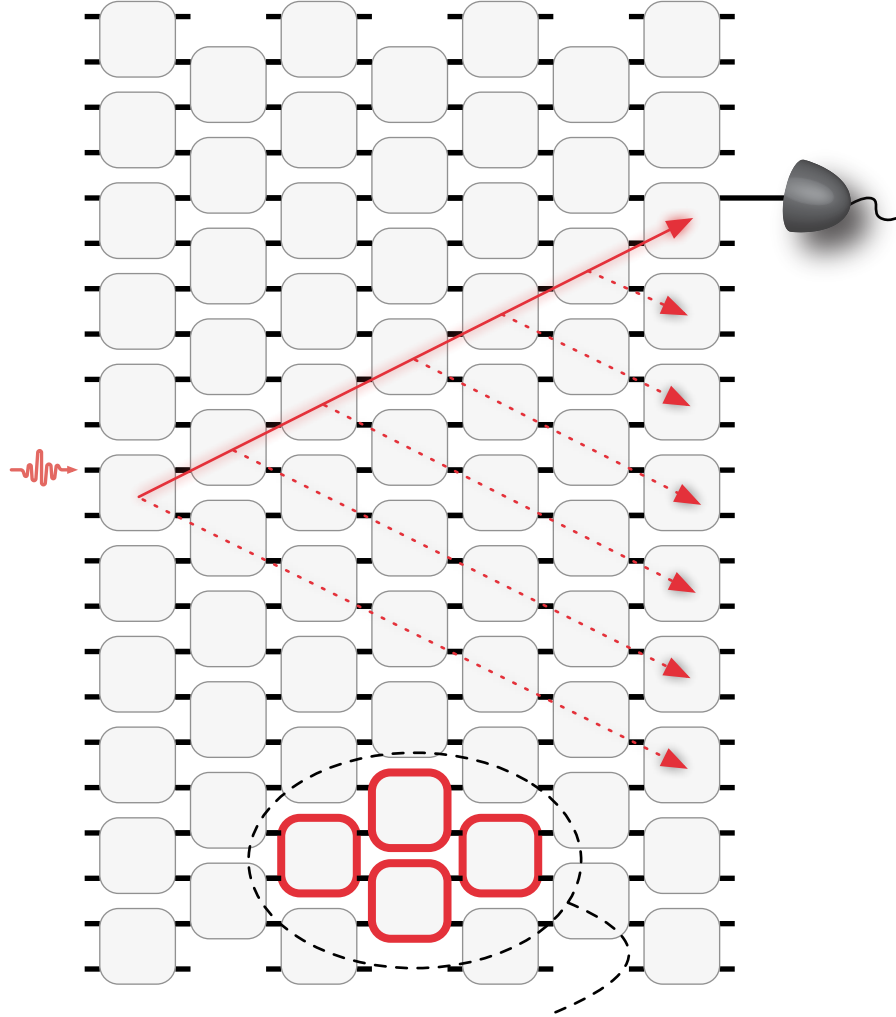

Meta-Interferometer

Figure 1: **Calibration procedure.** Input light is routed from an input mode along various wires (indicated by solid and dashed red arrows) through the PNP using a hill-climbing algorithm that maximizes the power at a given photodiode. Once a wire is routed, the internal phase of each MZI along that wire is swept while monitoring the power at the photodiode, giving both the phase offset and the phase vs. voltage curve for that RBS. A meta-interferometer is composed of four individual RBSs, as indicated by the solid red RBS grouping.

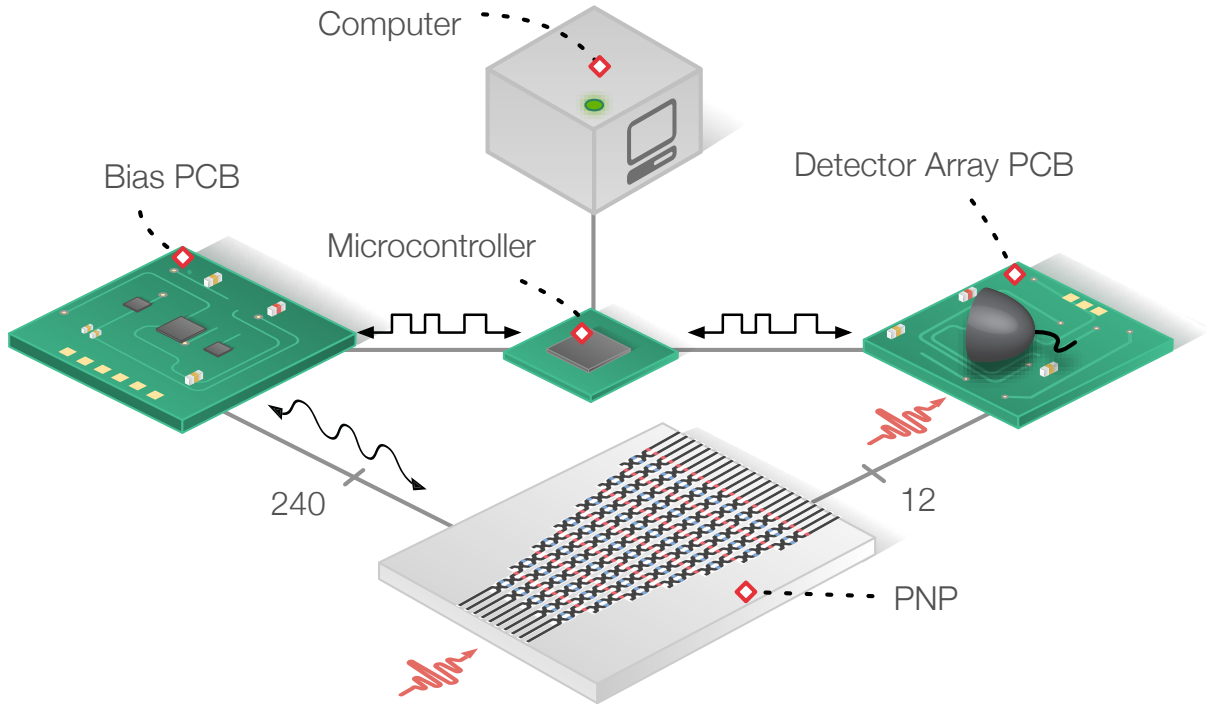

Figure 2: **Control and read-out setup.** A computer sends write/read commands to a microcontroller that communicates with the electronic control (Bias PCB) and optical read-out (Detector Array PCB) hardware. Before each complete reconfiguration, the Bias PCB issues a command to set all bias levels to 0 Volts and then load a 240 element 16-bit vector containing the bias settings for a desired unitary operation. After programming the PNP, the Detector Array PCB sequentially reads all optical outputs and reports the result as a 14 element floating-point vector. Since every other output waveguide is routed to the edge of the chip, we read the first half of the outputs and then the second set.

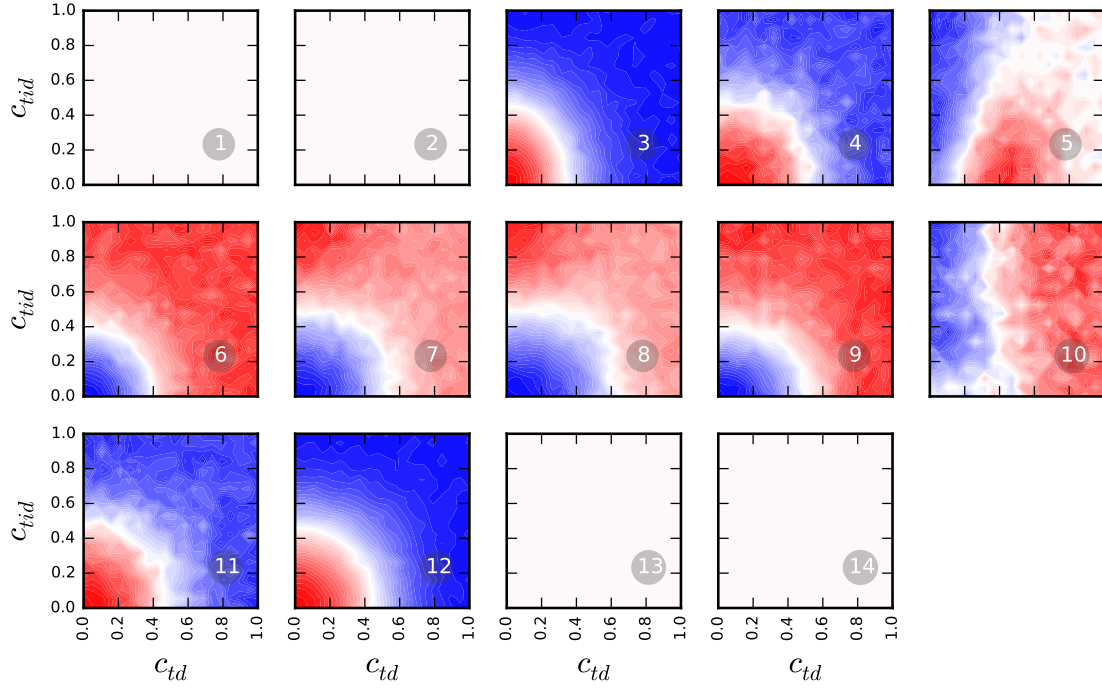

Figure 3: **Asymmetric transport.**  $\langle |\Psi(x, t_f)|^2 \rangle$  computer simulations for the PNP (mode numbers in bottom right corner). Here,  $\phi_1$  was modulated for throughout the array, which results in a quantum walk with an asymmetric response to static and dynamic disorder, specifically between modes 5 and 10.

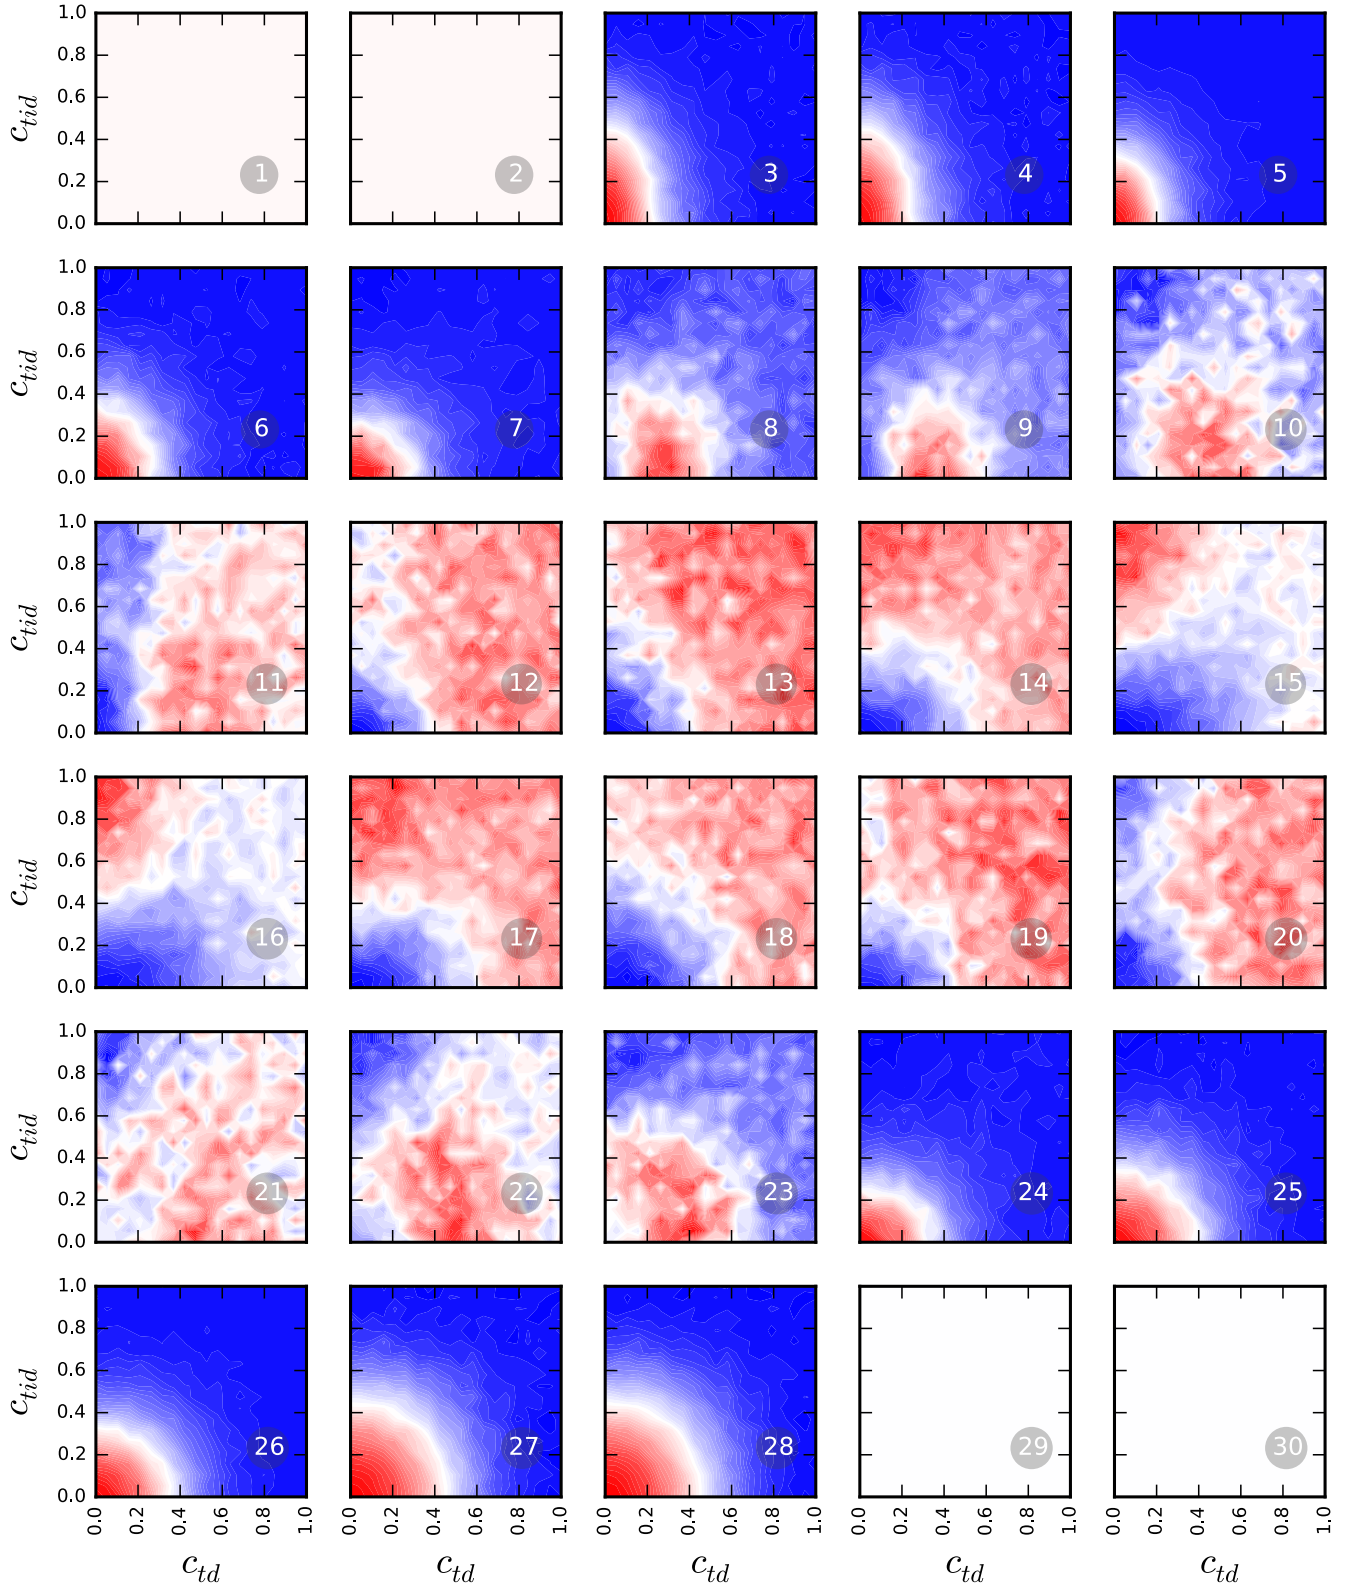

Figure 4: **Noisy transport simulations for a 15 time-step PNP.** 400 levels of disorder are simulated for a 15 time-step PNP. Mode numbers are indicated in the bottom right corner of each subplot. Modes 15 and 16 correspond to the MZI where light was injected and show maximal transport efficiency with  $c_{tid} = 1.0, c_{td} = 0.0$  (corresponding to Anderson localization). Modes 15 and 16 show minimal transport with  $c_{tid} = 0.0, c_{td} = 0.0$ , the case for which ballistic transport occurs. Modes 1, 2, 29, 30 are relatively constant across all levels of disorder due to the small number of possible paths that can constructively or destructively interfere on the edge of the light cone (as was seen in the experimental data in the main text). The outer modes 3, 4, 5, 6, 7 and 24, 25, 26, 27, 28 are all maximized during an ordered quantum walk.
